# Supplementary material for: Silicon Flexes Muscles: Giant Electrochemical Actuation in a Nanoporous Silicon-Polypyrrole Hybrid Material
Source: arXiv:2010.03878 ancillary file (2020-10-08)
Supplement: Supplementary file 1 [file PPy_pSi_actuation-V25_arxiv_org_Supplement_Figures_included.pdf]

# Supplement - Silicon Flexes Muscles: Giant Electrochemical Actuation in a Nanoporous Silicon-Polypyrrole Hybrid Material

Manuel Brinker,[1] Guido Dittrich,[1] Claudia Richert,[2] Pirmin Lakner,[3,4]
Tobias Krekeler,[5] Thomas F. Keller,[3,4] Norbert Huber[2] and Patrick Huber[1,3*]

[1]Institute of Materials Physics and X-ray Analytics ,
Hamburg University of Technology, 21073 Hamburg, Germany,
[2]Institute of Materials Research, Materials Mechanics,
Helmholtz-Zentrum Geesthacht, Geesthacht 21502, Germany,
[3]Centre for X-ray and Nano Science CXNS,
Deutsches Elektronen-Synchrotron DESY, Notkestraße 85, 22607 Hamburg, Germany,
[4]Physics Department,
University of Hamburg, 20355 Hamburg, Germany,
[5]Electron Microscopy Unit,
Hamburg University of Technology, 21073 Hamburg, Germany
[6]Centre for Hybrid Nanostructures CHyN,
University of Hamburg, 22607 Hamburg, Germany

[*]To whom correspondence should be addressed; E-mail: patrick.huber@tuhh.de.

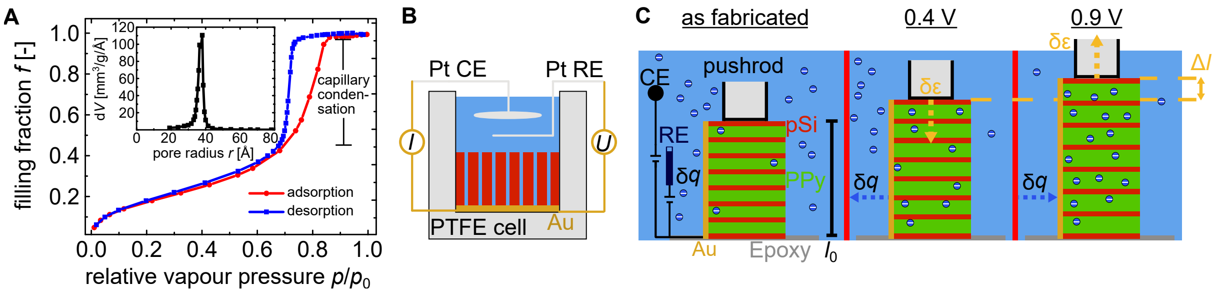


Figure S1: **Structural characterization by sorption isotherm, illustration of the polymerization cell and illustration of the electroactuation setup.** (**A**) Nitrogen sorption isotherm at $T = 77\,\mathrm{K}$ recorded for nanoporous silicon. Plotted is the volume filling fraction $f$ against the relative vapour pressure $p/p_0$. The inset depicts the resulting pore radius $r$ distribution. (**B**) Electrochemical cell for the polymerization of PPy in the pSi membrane. The membrane is contacted via a gold layer. The current is applied via a platinum counter electrode (CE) while the voltage is measured by a platinum wire acting as a pseudo reference electrode (RE). (**C**) Schematics of the electroactuation experiments. The pSi membrane filled with PPy is immersed in 1M perchloric acid ($HClO_4$) and contacted via the gold layer. The current is applied between a carbon counter electrode (CE) while the voltage is measured by a standard hydrogen reference electrode (RE). The right part symbolizes the case where a voltage of $0.9\,\mathrm{V}$ is applied and the anions are incorporated into the PPy resulting in the expansion of the sample. Vice versa, in the middle part a voltage of $0.4\,\mathrm{V}$ is applied and the anions are expelled followed by the subsequent contraction of the sample.
